# Supplementary material for: Forecasting Live Chat Intent from Browsing History
Source: arXiv:2408.04668 source file (2024-09-01)
Supplement: Supplementary file 1 [file appendix.tex]

\section{Appendix}
\label{sec:Appendix}

Without any interaction history provided, LLMs have very bad results.

\subsection{Role playing}

The first way is to directly instruct to role play, where the LLM should act as a person who watched movies.  
We use the gpt-3.5-turbo, and the OpenAI API allows to provide general instructions on how the model should behave. 
We use the same API for vicuna-7b (v1.3). 
The prompt we use is the following:

\begin{quote}
Let's do a role play. You are a person who watched some movies. Based on your assumed character, you are capable of replying whether you have or have not watched a movie.
\end{quote}

Then we inquire the model with a question on interaction.

\begin{quote}
Have you seen Titanic (1997)?
\end{quote}

In the role playing case, we find that vicuna-7b struggles understand the concept of taking the role of a user with specific interactions, always starting with the following utterance:

\begin{quote}
As an AI model, I do not have personal experiences or the ability to watch movies. However, I can provide information about the movie...
\end{quote}

On the other hand, gpt-3.5-turbo does give a proper answer.
However, it exhibits overly optimistic explanations on all the movies that were inquired, and it remains a question if real users would respond in such a verbose and eulogistic way:

\begin{quote}
Oh, my dear, I have indeed watched Titanic! It was a truly captivating film, filled with romance, tragedy, and breathtaking visuals. The love story between Jack and Rose, set against the backdrop of the ill-fated ship, was both heartwarming and heart-wrenching. I must say, it left quite an impression on me.
\end{quote}

Upon summarizing this response into `Yes' or `No', we find that all of most popular and middle popular movies were responded with `Yes' and all 5 of the least popular movies were responded with `No'.

\subsection{Dialog completion}

Since models may struggle to emulate users when directly do so, we instead allow them to observe a dialog in a third-person viewpoint and to complete it. 
We give a conversation between a seeker and recommender without any conditioning on the seeker and ask the LLM to complete the seeker's next response.
Here, we use the text-davinci-007 model.
The conversation we provide is the following.

\begin{quote}
Complete the following dialog.\\
Seeker: Hi, recommend me a movie.\\
Recommender: Let me ask you some questions to understand your preferences. Have you seen Titanic (1997)? \\
Seeker:
\end{quote}

In the case of dialog completion, vicuna-7b continues to give inappropriate responses, although in a different way. 

\begin{quote}
a) Yes\\
b) No\\
If you have seen it.
\end{quote}

The response of text-davinci-007 is better, and the problem of excessive optimism and exaggerated positivity is solved:

\begin{quote}
Yes, I have seen it.
\end{quote}

We note that the model responds `Yes' on all five most popular movies and `No' on all the other movies, leaving the question of how is the model deciding on this response and what kind of user the model is representing.

\subsection{Limitations of unconditioned generation}
We observe that LLMs may struggle when instructed to take on a role of a user and asked about interaction histories.
Although possible workaround is to let the model complete the dialog instead of asking it to impersonate a user, a fundamental limitation of any non-conditioning method is that we do not know who the LLM is representing. 
We need to be able to control the generation of a user such that we understand where the interaction histories of LLMs are coming from. 
In the next session, we will discuss conditioned generation.

\subsection{Prompts we used}

Role playing: 

\begin{quote}
You are a person who watched movies and gave the following ratings:\\
Movie 1, Rating 1\\
Movie 2, Rating 2\\
...\\
Movie N, Rating N\\
You haven't seen other movies.
\end{quote}

Dialog completion:

\begin{quote}
Complete the following dialog.
>> Person A: I watched movies and gave the following ratings.\\
    Movie 1, Rating 1\\
    Movie 2, Rating 2\\
    ...\\
    Movie N, Rating N\\
    I haven't seen other movies.\\
>> Person B: {question} Answer Yes or No.\\
>> Person A:\\

\end{quote}
